# Supplementary material for: AIR-Nets: An Attention-Based Framework for Locally Conditioned Implicit Representations
Source: arXiv:2110.11860 source file (2021-10-22)
Supplement: Supplementary file 1 [file faust_supp.tex]

\begin{figure*}[h]
    %\vspace{0.2cm}
    \begin{picture}(500,290)
        \put(0,0){\includegraphics[width=\linewidth]{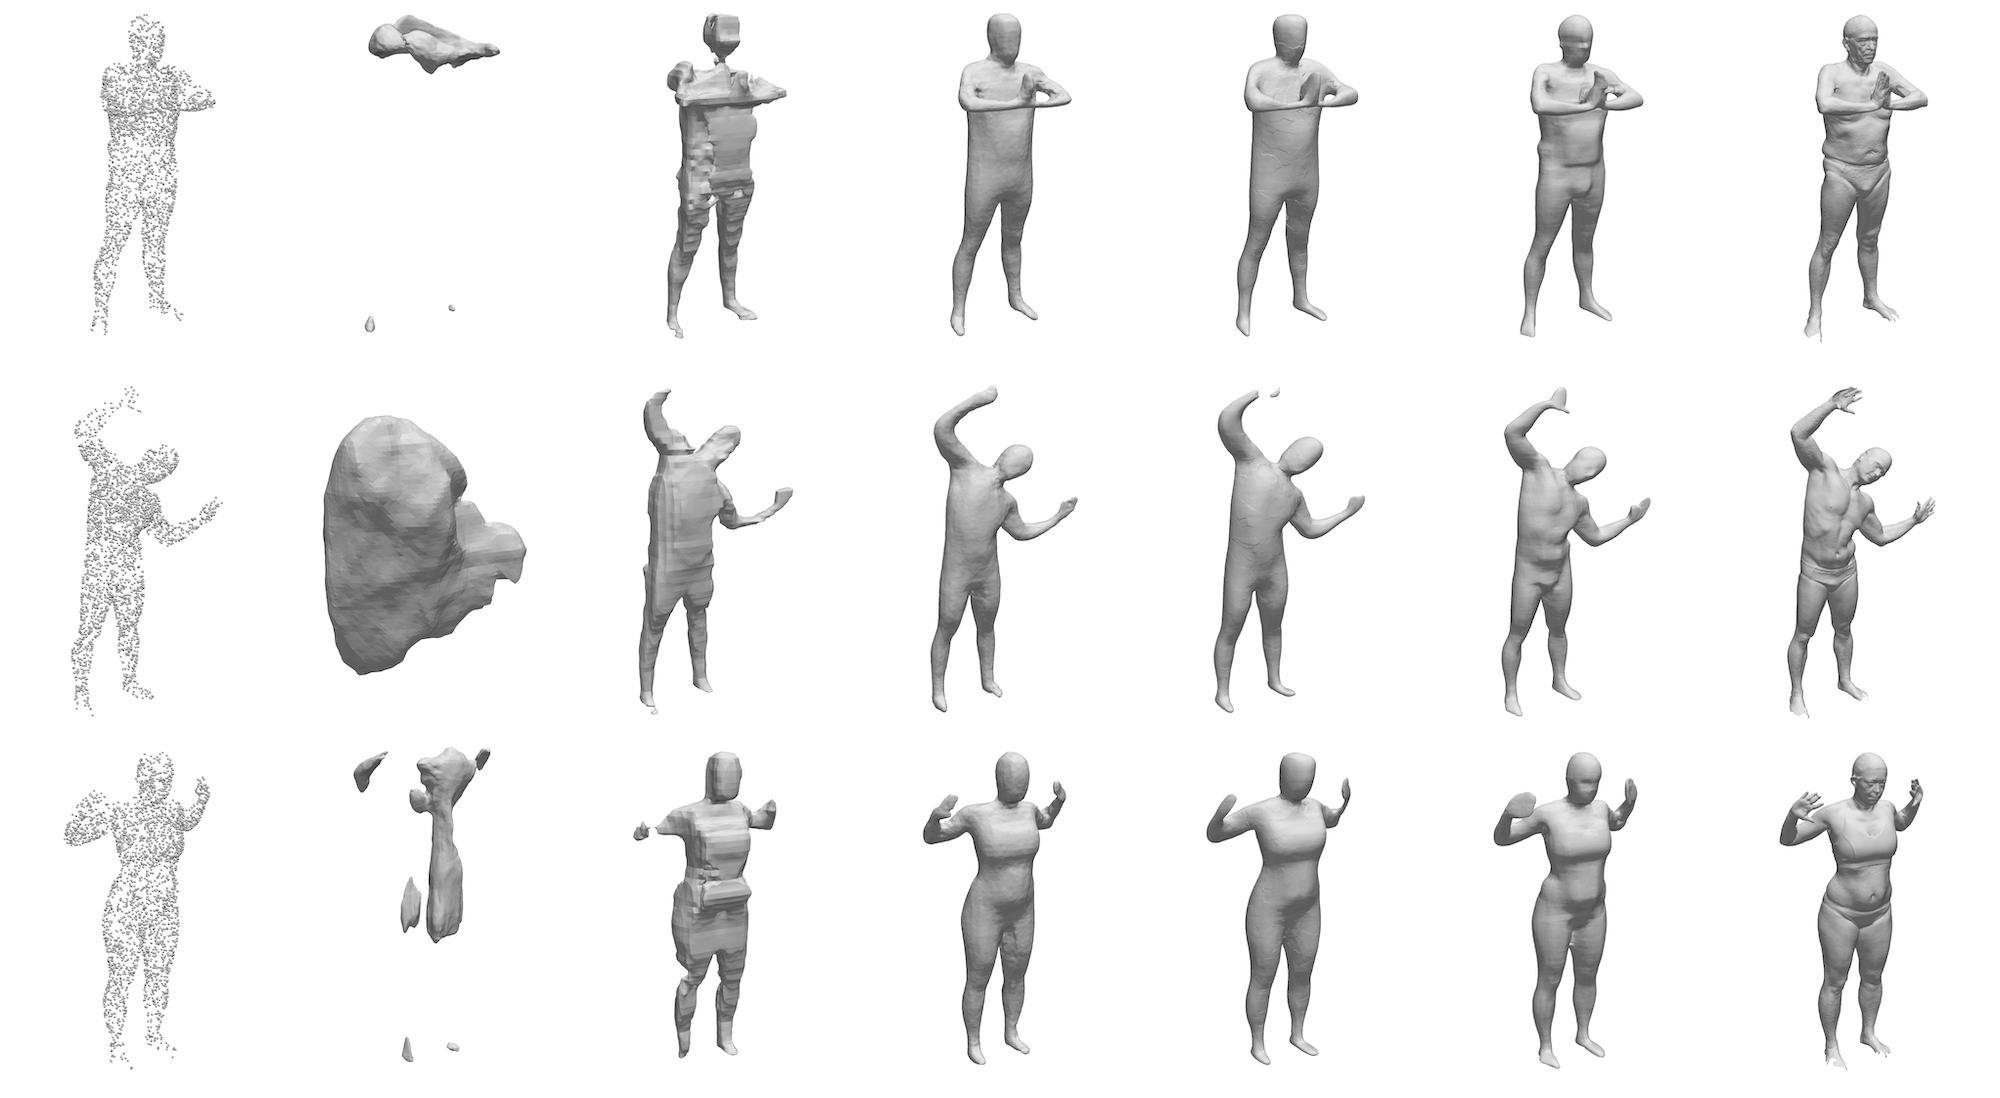}}
        \put(25,280){\small{Input}}
        \put(90,280){\small{$\text{ONet}_{\mathcal{D}_B}$}}
        \put(155,280){\small{$\text{ConvONet}_{\mathcal{D}_B}$}}
        \put(230,280){\small{$\text{IF-Net}_{\mathcal{D}_B}$}}
        \put(305,280){\small{$\text{Ours}_{\mathcal{D}_B}$}}
        \put(375,280){\small{$\text{Ours}_{\mathcal{D}_A}$}}
        \put(455,280){\small{GT}}
    \end{picture}
    \caption{\textbf{Zero-Shot 3D Reconstructions on FAUST.} We test the zero-shot generalization ability of models, that were trained in the dense setting on the ShapeNet dataset. Subscripts indicate which dataset the models were trained on. We chose the best performing dataset for each model and included both datasets for our model. Note that $\mathcal{D}_A$ does not contain any noise, while the FAUST data contains real measurement noise and holes, \eg see the feet of the ground trouth.}
    \label{fig:faust_supp}
\end{figure*}
